# Supplementary material for: Masked Unsupervised Self-training for Label-free Image Classification
Source: arXiv:2206.02967 source file (2023-03-10)
Supplement: Supplementary file 1 [file sec_appendix.tex]

\newpage

\begin{appendices}

\input{table/parameters.tex}

\end{appendices}
